# Supplementary material for: Procedure for 3D atomic resolution reconstructions using atom-counting and a Bayesian genetic algorithm
Source: arXiv:2105.05562 source file (2022-03-30)
Supplement: Supplementary file 1 [file supplementary.pdf]

# Supplementary Information

## Procedure for experimental reconstructions of 3D atomic structures from electron microscopy images using atom-counting and a Bayesian genetic algorithm

Annick De Backer[1,2], Sandra Van Aert[1,2,*], Christel Faes[3], Peter D. Nellist[4], and Lewys Jones[5,6,*]

[1]EMAT, University of Antwerp, Groenenborgerlaan 171, 2020 Antwerp, Belgium
[2]NANOlab Center of Excellence, University of Antwerp, Groenenborgerlaan 171, 2020 Antwerp, Belgium
[3]I-BioStat, Data Science Institute, Hasselt University, Hasselt, Belgium
[4]Department of Materials, University of Oxford, Parks Road, OX1 3PH Oxford, United Kingdom
[5]Advanced Microscopy Laboratory, Centre for Research on Adaptive Nanostructures and Nanodevices (CRANN), Dublin 2, Ireland
[6]School of Physics, Trinity College Dublin, The University of Dublin, Dublin 2, Ireland
[*]*E-mail: sandra.vanaert@uantwerpen.be,lewys.jones@tcd.ie*

| Parameter | Value |
|---|---|
| Acceleration voltage | 200 kV |
| Defocus $C_1$ | 0 nm |
| Spherical aberration $C_s$ | 0 nm |
| Convergence angle $\alpha$ | 22.48 mrad |
| Inner detector angle ADF | 52 mrad |
| Outer detector angle ADF | 248 mrad |
| Inner detector angle ABF | 9 mrad |
| Outer detector angle ABF | 21 mrad |
| FWHM of the source image | 1.0 Å |
| Debye-Waller factor | 0.384 Å$^2$ |
| Pixel size | 0.124 Å |
| Zone axis | [110] |
| Number of phonon configurations | 30 |

**Supplementary Table 1** – **Simulation settings.** Parameters for the frozen lattice simulation of a the Pt nanoparticle containing 587 atoms and Pt crystal in [110] zone axis up to 30 atoms thickness.

# Effective width of the normal distributions in the Gaussian mixture model

The estimated width $\sigma_{\mathrm{GMM}}$ should in principle take into account all dose-dependent and dose-independent uncertainties in the SCSs, including the limited electron dose and fluctuations in the SCSs from other effects such as the carbon support, different vertical onset of columns of the same number of atoms, intensity transfer between columns, and the influence of neighboring columns of different number of atoms [1]. At low doses $\sigma_{\mathrm{GMM}}$ is underestimated [2]. This can be easily observed by comparing the estimated width $\sigma_{\mathrm{GMM}}$ with the expected width from the dose-dependent uncertainty. The width $\sigma_{\mathrm{dose}}$ can be predicted by [3]:

$$\sigma_{\mathrm{dose}} = \sqrt{\mu_g/d}, \tag{1}$$

where $\mu_g$ corresponds to the expected SCS for a column containing $g$ atoms and $d$ equals the incident electron dose. $\sigma_{\mathrm{GMM}}$, based on the 30 noise realizations at each incident electron dose of the extensive simulation study presented in the main paper, and $\sigma_{\mathrm{dose}}$, based on Eq.(1), are shown in Fig. 1 to illustrate the underestimation at lower incident electron doses. In order to have a better estimation of the finite atom-counting precision at lower incident doses, an effective width $\sigma_{\mathrm{eff}}$ is therefore introduced which is the maximum of the two contributions:

$$\sigma_{\mathrm{eff}} = max(\sigma_{\mathrm{dose}}, \sigma_{\mathrm{GMM}}). \tag{2}$$

This $\sigma_{\mathrm{eff}}$ is a very good approximation for the true width of the underlying Gaussian mixture model since $\sigma_{\mathrm{dose}}$ will be dominant at doses lower than $2 \times 10^3 e^-/$Å$^2$ as demonstrated by Van Aert *et al.* [3]. From Fig. 1, it also clear that beyond this incident electron dose, the dose-independent width becomes more dominant.

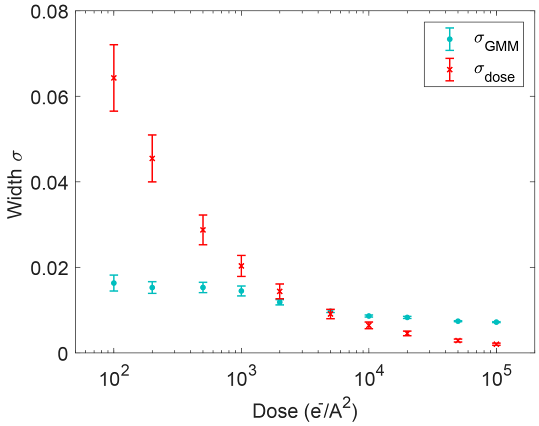


**Supplementary Figure 1 – Illustration of the width of the Gaussian components.** At lower incident electron doses the width $\sigma_{\mathrm{GMM}}$ is underestimated in comparison with the dose-dependent width $\sigma_{\mathrm{dose}}$. The 95% confidence intervals for the $\sigma_{\mathrm{GMM}}$ are computed using 30 noise realizations. For $\sigma_{\mathrm{dose}}$ the 95% confidence intervals indicate the spread due to thickness dependence of $\sigma_{\mathrm{dose}}$.

# References

[1] A. De Backer, G. T. Martinez, A. Rosenauer, and S. Van Aert. Atom Counting in HAADF STEM Using a Statistical Model-Based Approach: Methodology, Possibilities, and Inherent Limitations. *Ultramicroscopy*, 134:23–33, 2013.

[2] A. De wael, A. De Backer, L. Jones, P. D. Nellist, and S. Van Aert. Hybrid Statistics-Simulations Based Method for Atom-Counting from ADF STEM Images. *Ultramicroscopy*, 177:69–77, 2017.

[3] S. Van Aert, A. De Backer, L. Jones, G. T. Martinez, A. Béché, and P. D. Nellist. Control of Knock-On Damage for 3D Atomic Scale Quantification of Nanostructures: Making Every Electron Count in Scanning Transmission Electron Microscopy. *Physical Review Letters*, 122:066101, 2019.

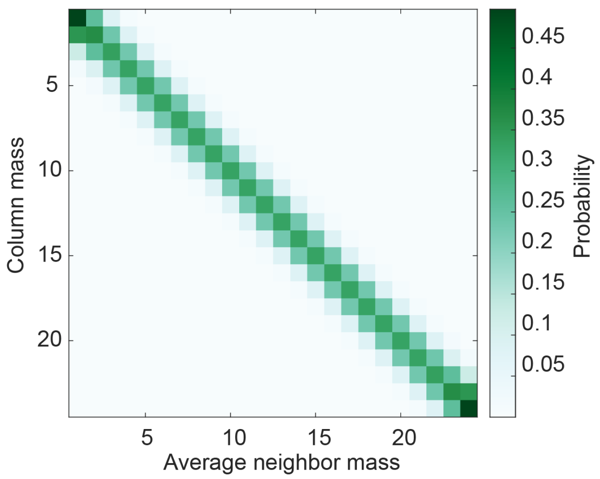


**Supplementary Figure 2 – Neighbor-mass probability matrix.** $p(g|NB_n)$ The average mass of the neighboring columns is shown on the $x$-axis and the column mass on the $y$-axis. The colormap illustrates the probabilities.

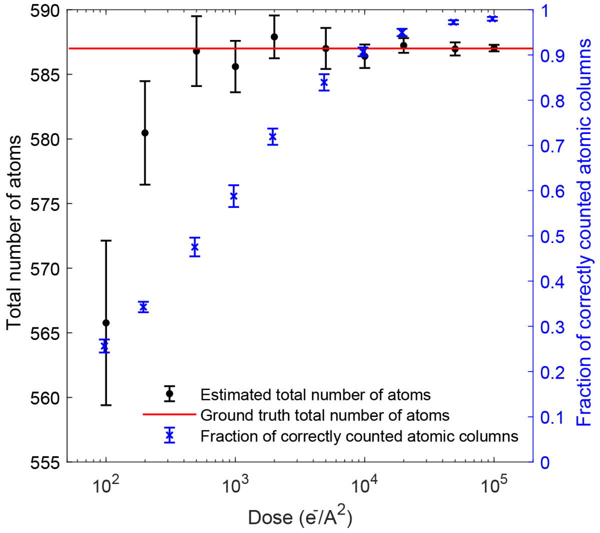


**Supplementary Figure 3 – Accuracy of the atom-counting results.** Estimated total number of atoms in the particle (left axis) and the fraction of atomic columns in which the number of atoms has been counted correctly (right blue axis). The error bars indicate $95\%$ confidence intervals. For the lowest doses, the total number of atoms is slightly underestimated and as expected the fraction of correctly counted atomic columns decreases when the incident electron dose decreases. These atom-counting results are used as an input for our Bayesian genetic algorithm.

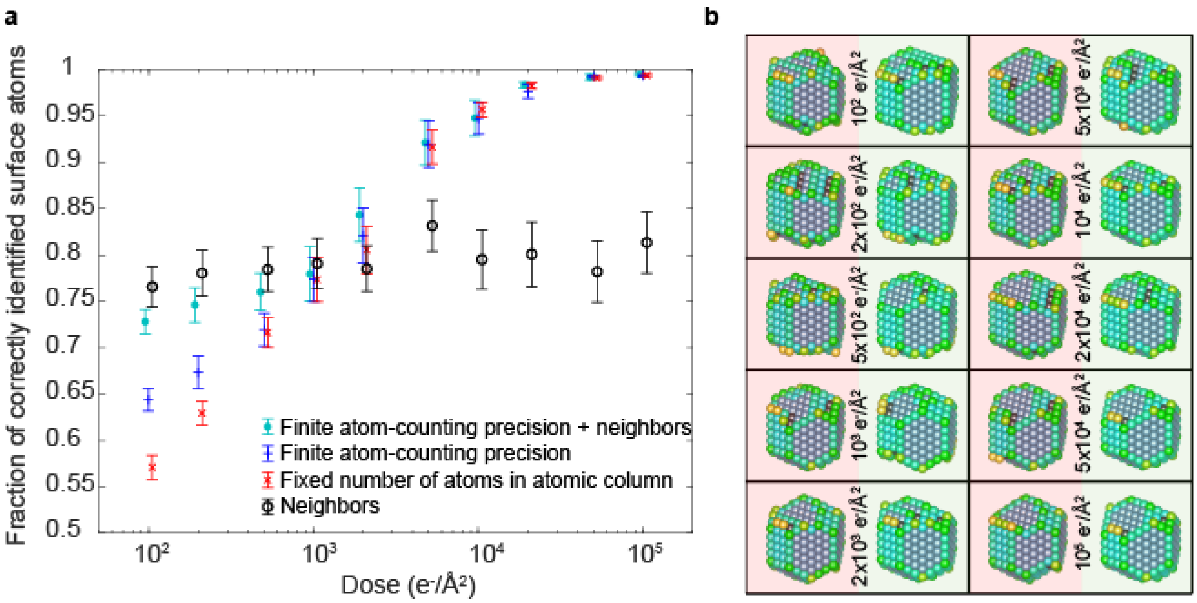


**Supplementary Figure 4 – Results for the reconstructions using the neighbor-mass relations only. a** Fraction of the surface atoms that are correctly defined in 3D with 95% error bars when including both the finite atom-counting precision and neighbor-mass relations (light blue), the finite atom-counting precision only (dark blue), and the neighbor-mass relations only (black) as prior knowledge. As a reference the results when using a fixed number of atoms in a column are also displayed. **b** Visualization of the reconstructed 3D atomic models represented by the lower bound (red background) and upper bound (green background) of a 80% prediction interval for the reconstructions when using the neighbor-mass relations only.

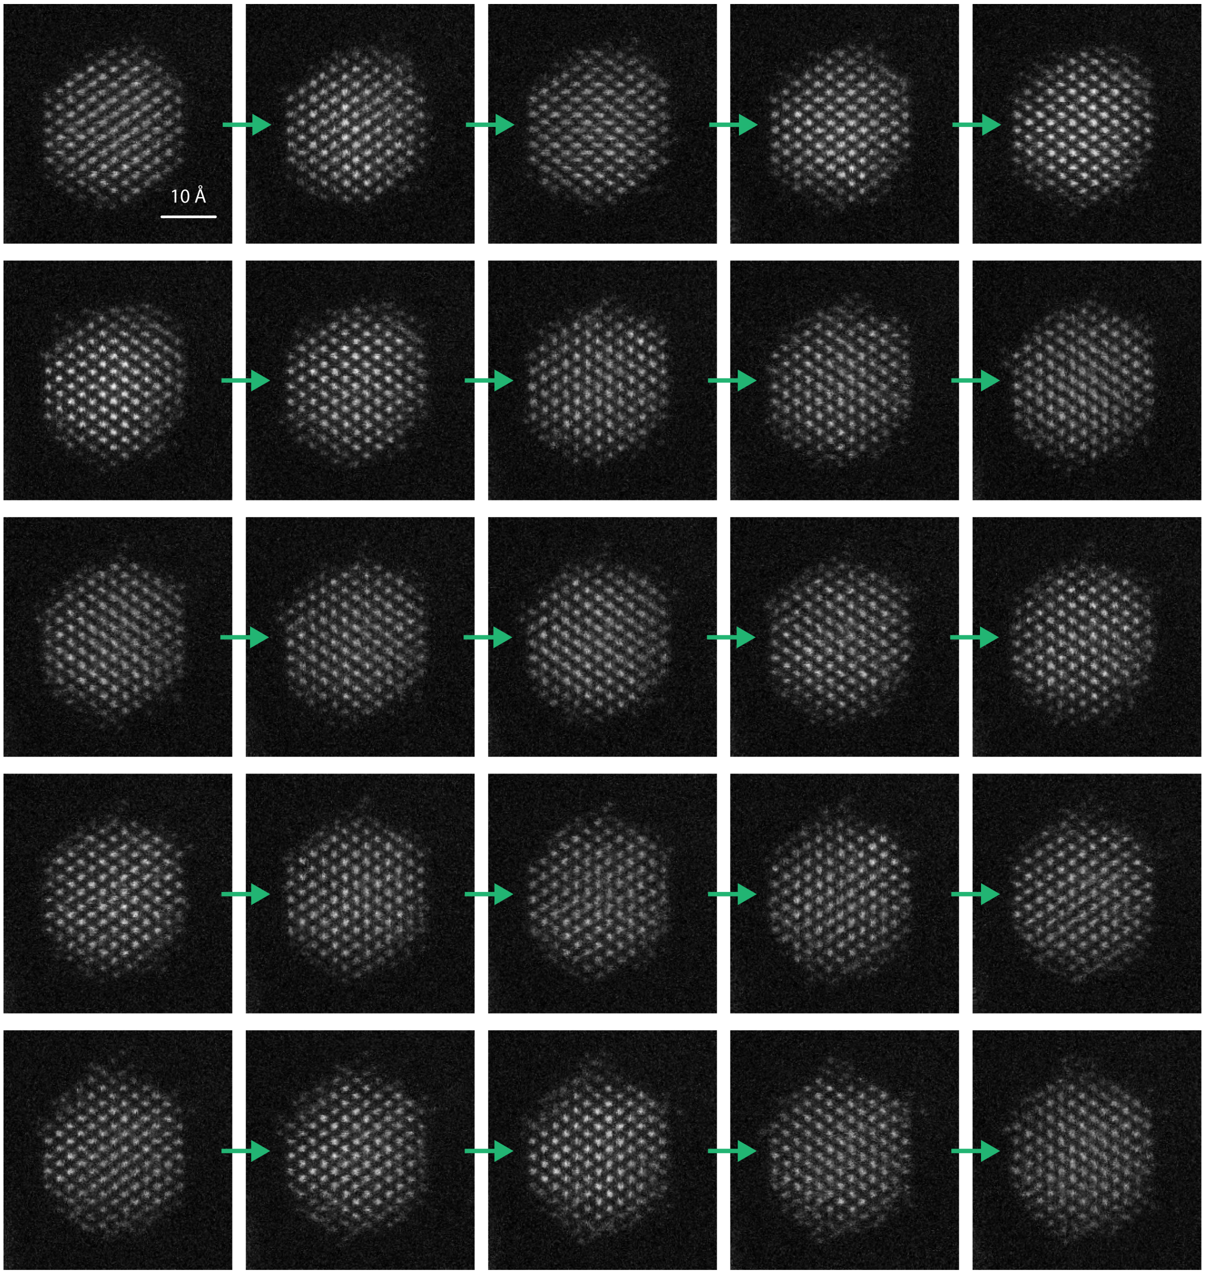


**Supplementary Figure 5 – Experimental ADF STEM time-series of the Pt nanoparticle.** Time progresses along the rows.

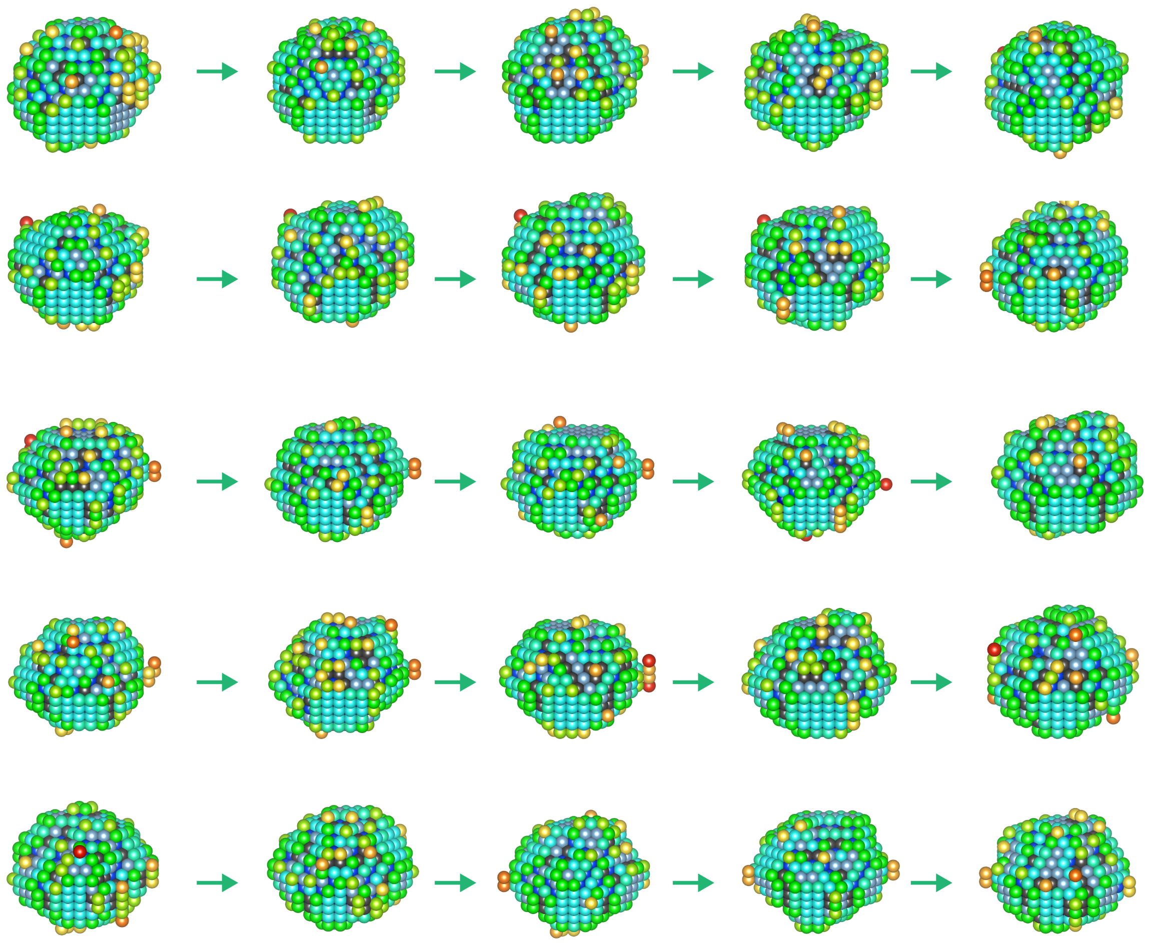

**Supplementary Figure 6 – 3D atomic models.** Reconstructions obtained by the Bayesian genetic algorithm including the finite atom-counting precision and neighbor-mass relations as prior knowledge for the time series from Figure 5.

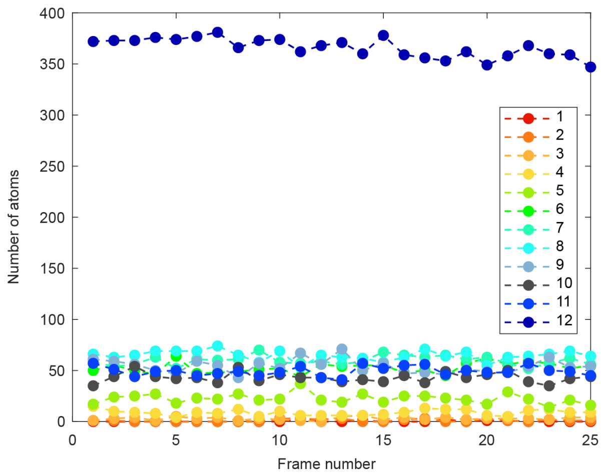


**Supplementary Figure 7 – Atomic coordination number analysis.** The number of atoms with the a specific coordination number are shown for the time series of the Pt nanoparticle.
